# Supplementary material for: Retrieval-Pretrained Transformer: Long-range Language Modeling with Self-retrieval
Source: arXiv:2306.13421 source file (2024-07-21)
Supplement: Supplementary file 1 [file appendix.tex]

% \subsection{Additional details regarding neighbour augmentation}
% \label{app:additional_cca}

% Like RETRO,  retrieved representations are further augmented by applying cross-attention over the query chunk. Specifically, our \textit{augmented retrieved representation} $C^{\textbf{a}}_{i,k}$ for neighbor $k$ of chunk $c_i$ is obtained by applying cross attention where the retrieved representation $C_{i,k}$ serves as the query, and the query chunk $c^{\textbf{q}}$ representation from the lower decoder serves as the key and value. This is since integrating information from $c^\textbf{q}$ would help the retrieved neighbours represent information relevant for generating $c^{\textbf{t}}$.
